# Supplementary material for: Disordered dimer state in electron-doped Sr$_{3}$Ir$_{2}$O$_{7}$
Source: arXiv:1608.03565 ancillary file (2016-08-11)
Supplement: Supplementary file 1 [file Supplementary_Material.pdf]

# Supplementary Material

*Disordered dimer state in electron-doped $Sr_3Ir_2O_7$*

Tom Hogan, Rebecca Dally, Mary Upton, J. P. Clancy, Kenneth Finkelstein,
Young-June Kim, M. J. Graf, and Stephen D. Wilson

## I. Resonant Inelastic X-Ray Scattering (RIXS) Setup:

Resonant inelastic x-ray scattering data were collected on the insertion device beamline 27-ID-B at the Advanced Photon Source at Argonne National Laboratory. Samples were mounted to an aluminum fixture with a small amount of GE varnish, which was then connected to a closed cycle refrigerator (CCR). In order to maximize signal intensity a radiation shield was not used. Instead, only a Be-domed vacuum shroud was used which limited the base temperature to 40 K. Scattering measurements were conducted primarily within the (H, K, 26.5) plane, with the crystal aligned via the **Q**=(0, 0, 20) and **Q**=(1, 1, 20) Bragg reflections (indexed in the approximate *I4/mmm* tetragonal space group). A double crystal diamond-111 monochomator was positioned before a channel cut Si-448 monochromator, with $E_i$ set to the Ir $L_3$ edge value (11.215 keV). $E_f$ was measured with a diced spherical Si-448 analyzer and a Dectris mythen detector. After alignment of the incident optical components, the sample scattering angle $2\theta$ was set to 20° (vertical), and an energy scan was taken to measure the elastic line from two pieces of scotch tape. The full width at half maximum (FWHM) of the resulting peak provides a metric for the energy resolution of the measurement. This feature is fit below with a pseudo-Voight function.

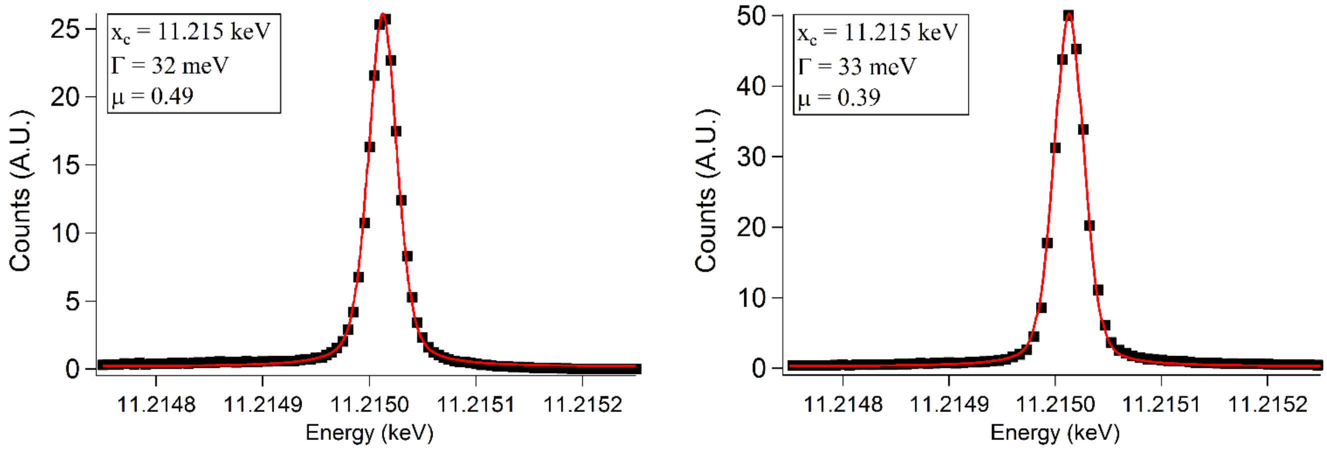


*Fig. S1: Pseudo-Voight fits of incoherent elastic scattering after spectrometer alignment at the start of experiments measuring the x=0.07 (left panel) x=0.02 (right panel) samples. μ denotes the shape parameter, $x_c$ the center, and Γ the width of the peaks.*

## II. RIXS Spectral Fitting Routine and Constraints

Energy spectra were fit using the following components: (1) an overall constant background term, (2) an elastic line fit to a pseudo-Voigt function, (3) a small linear background on the x-ray energy loss side typically associated with a particle-hole continuum, and (4) a series of four Lorentzian peaks multiplied by the Bose population factor and associated with magnetic (*M*, *M**) and *d-d* excitations (*D*). These peaks were symmetrized to the energy gain side of the spectrum using detailed balance; however their contributions are suppressed due to weighting by the Boltzmann factor (where $T_{measurement}$ = 40 K << $\Delta E_{resolution}/k_B$ = 371 K).

The fitting routine was executed in four steps, the first three of which identified a workable set of starting parameters for a full fit to the data. These steps were: (1) the energy gain side of the spectrum was fit to a pure pseudo-Voight function and constant background term to extract the elastic line's profile. (2) the parameters

associated with features in the region -1500 < ΔE < -500 meV were then added to the refinement. This consisted of *d-d* excitations (*D*-peaks) as well as a small linear background term. (3) These high energy and elastic peak parameters were then fixed, and the low energy *M* and *M** peaks (-500 < ΔE < 0 meV) were added and allowed to refine. (4) Having identified these parameters as a starting point, as a final step, all parameters are then refined simultaneously for the final fits shown in the main text and supplementary materials. Fits assumed that the *M** peak was present in all spectra, that its amplitude should be less than that of the *M* peak, and that its width should be of the same order of the *M* peak.

## III. Hamiltonian and Dispersion Fit Results

For completeness, we reproduce the spin Hamiltonian and bond operator (BO) derived dispersion relation from Moretti Sala *et al.* [21].

$$H = J_1 \sum_{\langle i,j\rangle,l} \left[\cos(2\theta)\, \boldsymbol{S}_{li} \bullet \boldsymbol{S}_{lj} + 2\sin^2(\theta)\; S_{li}^z S_{lj}^z - \varepsilon_i \varepsilon_l \sin(2\theta) \left(\boldsymbol{S}_{li} \times \boldsymbol{S}_{lj}\right) \bullet \hat{e}_z \right]$$
$$+ J_c \sum_i \boldsymbol{S}_{1i} \bullet \boldsymbol{S}_{2j} + J_2 \sum_{\langle\langle i,j\rangle\rangle,l} \boldsymbol{S}_{li} \bullet \boldsymbol{S}_{lj} + J_3 \sum_{\langle\langle\langle i,j\rangle\rangle\rangle,l} \boldsymbol{S}_{li} \bullet \boldsymbol{S}_{lj}$$

Reproduced from Eq. (1) in Ref. 1, the exchange constants $J_1$, $J_c$, $J_2$, and $J_3$ are depicted in Fig. 1 in the main text of this work. The parameter $\theta$ is a measure characterizing the degree of anisotropy of the interactions. The dispersion relation associated with the BO treatment of the above Hamiltonian is given by:

$$\omega_{\boldsymbol{q},\alpha} = \sqrt{A_{\boldsymbol{q},\alpha}^2 - \left|B_{\boldsymbol{q},\alpha}\right|^2}$$

Where α indicates the longitudinal (z) and degenerate transverse (τ = x,y) modes, the constituent functions are:

$$A_{\boldsymbol{q},z} = 4J_1 \left[\sin^2(2\chi)\left(1 - \frac{J_2}{J_1} - \frac{J_3}{J_1}\right) + \frac{J_c}{4J_1}\cos(2\chi)\right] + \frac{J_1}{2}\left[\cos^2(2\chi)\,\gamma_{\boldsymbol{q}} + \frac{J_2}{J_1}\delta_{\boldsymbol{q}} + \frac{J_3}{J_1}\phi_{\boldsymbol{q}}\right]$$
$$B_{\boldsymbol{q},z} = \frac{J_1}{2}\left[\cos^2(2\chi)\gamma_{\boldsymbol{q}} + \frac{J_2}{J_1}\delta_{\boldsymbol{q}} + \frac{J_3}{J_1}\phi_{\boldsymbol{q}}\right]$$
$$A_{\boldsymbol{q},\tau} = 2J_1\left[\frac{J_c}{2J_1}\cos^2(\chi) + \sin^2(2\chi)\left(1 - \frac{J_2}{J_1} - \frac{J_3}{J_1}\right)\right] + \frac{J_1}{2}[\cos(2\theta)\cos(2\chi)]\gamma_{\boldsymbol{q}} + \frac{J_2}{2}\delta_{\boldsymbol{q}} + \frac{J_3}{2}\phi_{\boldsymbol{q}}]$$
$$B_{\boldsymbol{q},\tau} = \frac{J_1}{2}\,[\cos(2\theta) - i\sin(2\theta)\sin(2\chi)]\gamma_{\boldsymbol{q}} + \frac{J_2}{2}\cos(2\chi)\,\delta_{\boldsymbol{q}} + \frac{J_3}{2}\cos(2\chi)\,\phi_{\boldsymbol{q}}$$

Further parameterizations of these functions are defined as:

$$\gamma_{\boldsymbol{q}} = 2\left(\cos q_x + \cos q_y\right)$$
$$\delta_{\boldsymbol{q}} = 2\left[\cos\left(q_x + q_y\right) + \cos\left(q_x - q_y\right)\right]$$
$$\phi_{\boldsymbol{q}} = 2\left(\cos 2q_x + \cos 2q_y\right)$$
$$\chi = \frac{1}{2}\cos^{-1}\left(\frac{J_c}{4(J_1 - J_2 - J_3)}\right)$$

The exchange parameters obtained by fitting *M* peak energies to the above dispersion relations (as shown in Fig. 3 in the main text) are summarized in Table S1 alongside corresponding values for the parent compound as reported in Ref. [1]. Uncertainties reported in the exchange parameters extracted from fits to the dispersion are often artificially low, and an alternate, empirical, uncertainty bound is ~5% of the exchange constant.

|  | $x = 0$<br>*Moretti Sala, et al. [Ref. 1]* | $x = 0.022$<br>*This Work* | $x = 0.071$<br>*This Work* | **Units** |
|---|---|---|---|---|
| $J_1$ | 26 | 37.7 ± 0.4 | 29.1 ± 0.7 | meV |
| $J_2$ | -15 | -14.0 ± 0.3 | -17.0 ± 0.6 | meV |
| $J_3$ | 6 | 4.8 ± 0.3 | 5.2 ± 0.6 | meV |
| $J_c$ | 90 | 87.6 ± 1.1 | 80.1 ± 2.3 | meV |
| $\theta$ | 37 | 41.2 ± 0.7 | 37.2 ± 1.7 | degrees |

*Table S1: Summary of refined magnetic exchange parameters for x=0.02 and x=0.07 samples compared with the parent x=0 system as reported in Ref. 1. Note that errors are extracted from the non-linear least squares fitting routine and are artificially low.*

## IV. Resonant Inelastic X-ray Scattering: *L*-dependence of *M* and *M** peaks

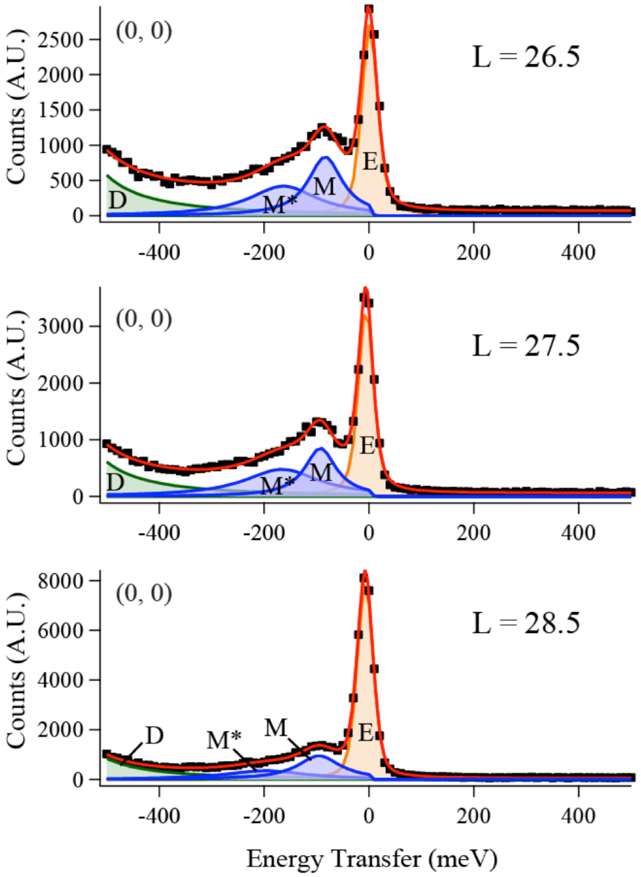


*Fig. S2: Raw data and fits of energy scans collected at various L values along fixed Q=(0,0,L) for the x=0.07 sample. Data shown here were collected at 40 K.*

In order to investigate the out-of-plane (L-dependent) dispersion of the magnon peaks a series of spectra were collected for various *L* values at a fixed in-plane momentum transfer of **Q**=(0,0). This in-plane position also corresponds to the wave vector where the longitudinal mode in the parent material had dispersed far away from the principal magnetic peak [1]. Spectra collected at **Q**=(0, 0, *L*) positions for the *x*=0.07 sample are shown in Fig. S2. Aside from the increase in the elastic peak (associated with increase in Thompson scattering caused by the scattering angle deviating from the near-90° condition at *L* = 26.5) we note that there is no additional feature resolved that may be attributed to a longitudinal branch. Subsequent fitting of these spectra (Fig. S2) demonstrate that the data are fully reproduced by fits employing only the *E*, *M*, *M** and *D* features described in the main text. The resulting fit peak areas and energies of the *M* peaks are plotted in Fig. S3. Both are *L*-independent within error.

The failure to resolve the longitudinal mode is likely due to the dopant induced overdamping of the spin excitations. The rapid decrease in excitation lifetimes (shown in Fig. S3) with increasing La-content precludes any subtle features from being conclusively extracted from the data. The predicted intensity of the longitudinal mode relative to transverse modes [1] is illustrated in the left panel of Fig. S3. The right panel of Fig. S3 depicts the lifetime broadening of the *M* peaks as La content is increased from the insulating *x*=0.02 sample to the metallic *x*=0.07 sample. The weak momentum dependence of the *M* peaks inverse lifetime values is also illustrated.

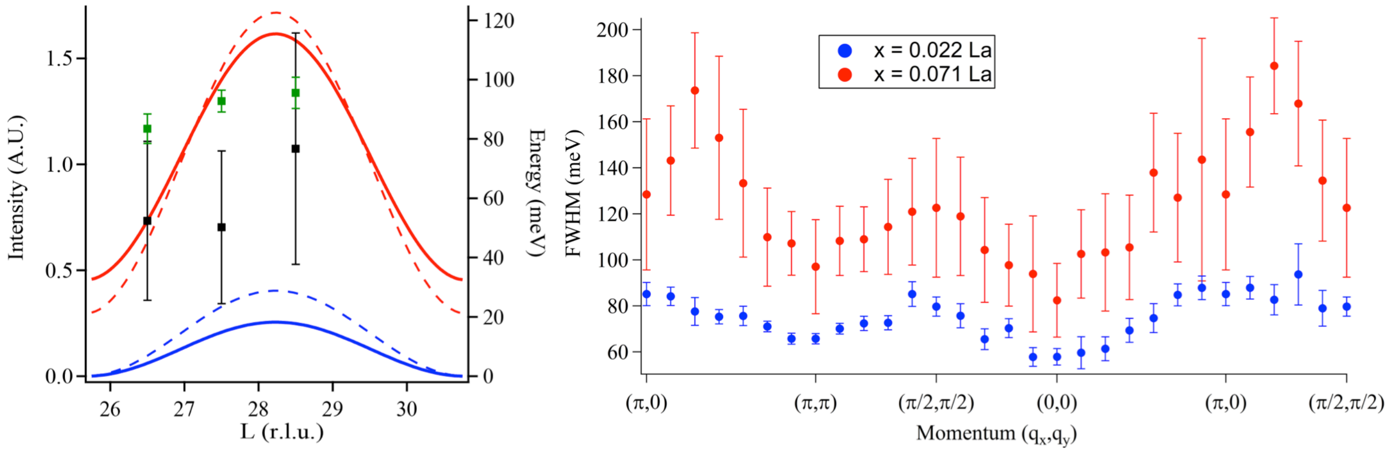


*Fig. S3: (Left panel) Calculated L-dependence for intensities of the transverse (red) and longitudinal (blue) modes at fixed momentum transfer* ***Q****=(0,0,L). Dashed lines indicate calculation for the parent using parameters reported in [1]; solid lines were calculated using exchange constants derived from fits to the M-dispersion of the x=0.07 sample in this work. Black squares are the spectral weight of the M feature in Fig. S2, normalized to the model curve at L=26.5 for clarity. Green squares, corresponding to the right axis, indicate the center of the M peak. (Right panel) M-peak widths as a function of in-plane momentum transfer ($Q_c$ fixed at L=26.5). Red symbols show fit values for the x=0.07 sample and blue symbols show values for the x=0.02 sample.*

## V. Additional Representative RIXS Spectra

Additional representative RIXS spectra and fits collected at select high symmetry points are provided below.

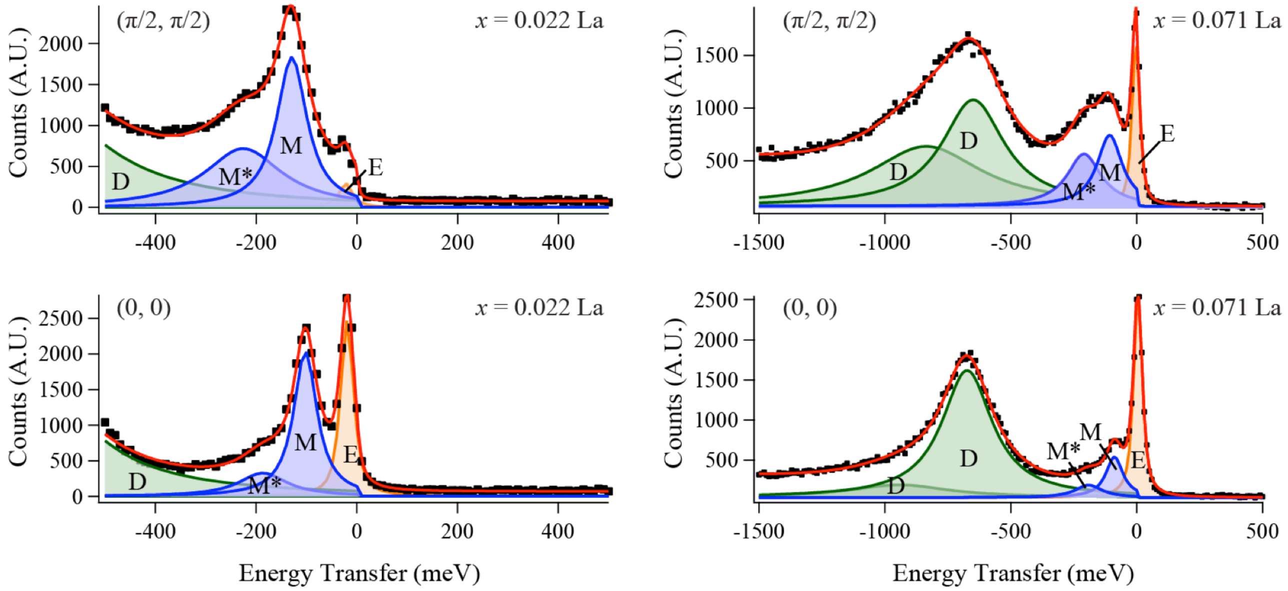


*Fig. S4: Additional representative spectra and corresponding fits are shown for the Q=(π/2, π/2) and Q=(0, 0) in-plane momentum points for the x=0.02 (left panels) and x=0.07 (right panels) samples. Data were collected at T=40K at a fixed L=26.5.*

## VI. Alternate Analysis of Nondegenerate (π, π) and (0,0) Gap Energies

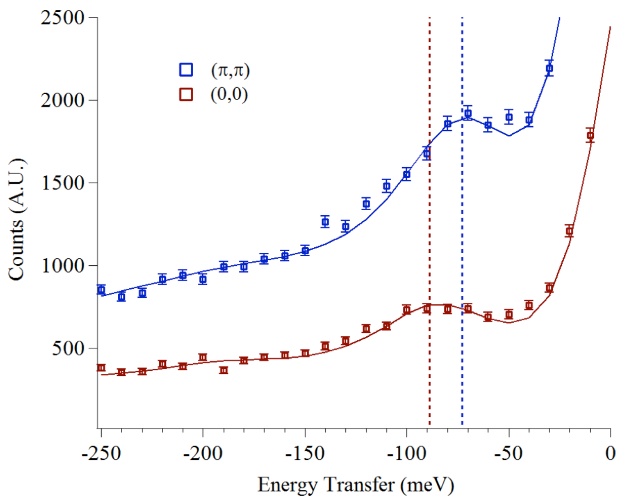


*Fig. S5: Zoom in of raw RIXS data collected at* $\boldsymbol{Q}_{HK}=(\pi,\pi)$ *(blue squares) and* $\boldsymbol{Q}_{HK}=(0,0)$ *(red squares). Solid lines are the combined fits to the data as described in the main text. Dashed vertical lines denote the energy centers for M peaks in each scan.*

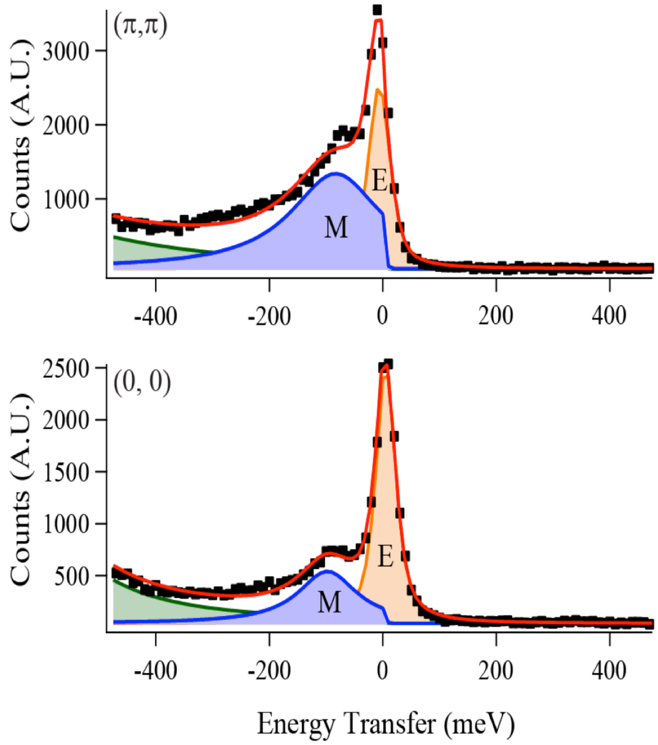


*Fig. S6: Fitting of energy scans at (π,π) and (0,0) using a single peak to parameterize* $(M+M^*)$ *and capture the magnetic spectral weight from an assumed convolution of M and M* peaks for the x = 0.07 sample*

To better illustrate the inequivalent energies of M peaks measured at the zone center $\mathbf{Q}_{HK}=(\pi, \pi)$ and $\mathbf{Q}_{HK}=(0, 0)$ positions, a zoomed in comparison of the raw data of energy scans and corresponding fits for the $x$ = 0.07 sample is plotted in Fig. S5. Inspection of the raw data shows that there is a shift in the total spectral weight to lower energies at the (π, π) position relative to the zone boundary at (0,0). Dashed lines mark the fitted peak positions for the M features in each spectrum reported in the main text Fig. 3 (b). While this 15 meV difference is smaller than the absolute energy resolution of the instrument, the systematic, relative, shift in the energies of M-peaks can be isolated outside the uncertainty of the fitting procedure (~5 meV).

Due to the large overlap between the two M and $M^*$ peaks and the inherently broadened nature of these peaks in the spectra of doped samples, an alternative limit should be considered. Namely, the limit where the two peaks are sufficiently convolved together to an extent that it is no longer meaningful to distinguish between them. In this limit, they should be treated as only one (M+M*) peak in the spectrum, whose total spectral weight will generate a muted form of the magnon dispersion. Energy differences in this convolved, single peak, scenario provide a worst case limit for our ability to parameterize the spin spectrum and gap values at the zone center and zone boundary positions.

Fitting the data to a single (M+M*) Lorentzian peak in this way is plotted in Fig. S6 and provides considerably poorer fits than an approach distinguishing between M and $M^*$ peaks (for comparison see main text Fig. 2 (c)). Nevertheless, the parameterization of this unbiased check still shows an identical energy difference between the spectral weight at the (π, π) and (0,0) positions. Fit values for the two approaches are listed below.

| | $\mathbf{Q}_{HK}$ = (π,π) | $\mathbf{Q}_{HK}$ = (0,0) | ΔE |
|---|---|---|---|
| $(M + M^*)$ fit convolved | 83 ± 6 meV | 98 ± 5 meV | 15 meV |
| $M$ and $M^*$ fit individually | 73 ± 4 meV | 89 ± 4 meV | 16 meV |

## VII. Resonant Elastic X-Ray Scattering (REXS) Setup and Additional Results

The resonant elastic x-ray diffraction data were collected on the bending magnet beamline C1 at the Cornell High Energy Synchrotron Source (CHESS) at Cornell University. The sample was mounted to a copper post with a small amount of GE varnish, which was then connected to a 4 K CCR employing Be domes for the radiation shield and vacuum shroud. Scattering measurements were conducted in the (H, H, L) scattering plane, and samples aligned using the (0, 0, 10) and (1, 1, 10) Bragg reflections (using the approximate tetragonal *I4/mmm* indexing). Elastic data reported here was collected at the Ir $L_3$ edge (11.218 keV) utilizing a PG-006 crystal for polarization analysis and a NaI detector.

## VIII. Additional REXS Data: Scans Along High Symmetry Directions for *x*=0.05

When no signal was found at the nominal magnetic wave vector **Q**=(0.5, 0.5, 18) in the σ-π channel, additional wider scans along high-symmetry directions were made in an attempt to perform a broader search of alternate positions in reciprocal space. In Fig. S7 these scans have been normalized to a monitor, background subtracted, and offset from zero for clarity in order to demonstrate that no magnetic correlations were observed. Data points represent count times of at least three minutes per point. The comparison of the (0.5, 0.5, 19) peak, a weak structural reflection shown at (1/50) scale in the main text Fig. 4 (b), was measured in the σ-σ channel and found to be nonresonant, as shown in Fig. S8 below.

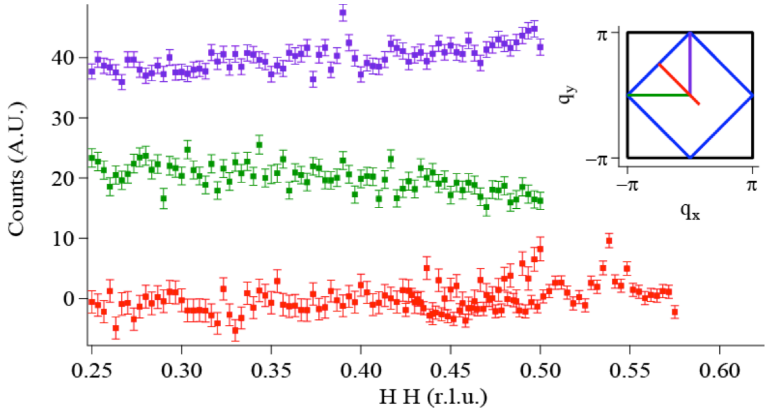


*Fig. S7: Scans along high symmetry directions of the magnetic zone. Curve colors correspond to the direction of the cut shown in the inset map of reciprocal space using the notation, employed throughout the text, corresponding to a tetragonal unit cell.*

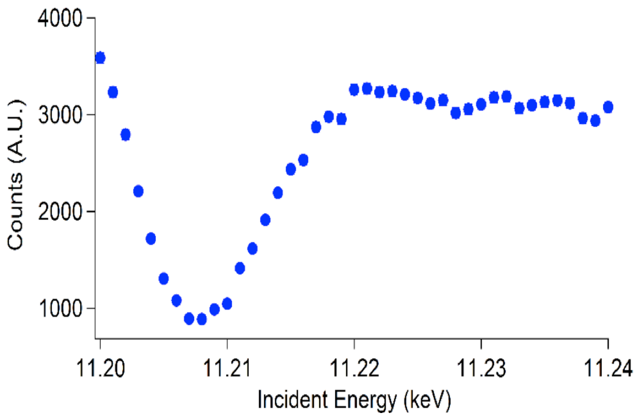


*Fig. S8: Energy scan in the σ-σ channel at the **Q**=(0.5, 0.5, 19) peak position showing a signature of the Ir-$L_3$ absorption edge and no resonant enhancement.*

## IX. Additional REXS Data: Data for *x*=0.023 and Ordered Moment Upper Bound for *x*=0.05

An AF ordered *x*=0.023 sample was also explored via REXS. Radial scans were performed at 7 K through the **Q**=(0.5, 0.5, 18) and **Q**=(0.5, 0.5, 19) positions in the σ–π and σ–σ scattering channels respectively. Data from these radial scans were normalized to a common monitor, constant background terms were subtracted, and are shown in Fig. S9. Here both the antiferromagnetic Bragg reflection at (0.5, 0.5, 18) and the weak structural peak at (0.5, 0.5, 19) are apparent. These data give a relative measure of the intensities of the (0.5, 0.5, 19) and (0.5, 0.5, 18) peaks in a control sample whose ordered moment is known to be $m_{AF}$ ~ 0.31 $\mu_B$ [25]. The corresponding scans performed on an *x*=0.05 sample are plotted in the main text's Fig. 4 (b) and can now be

compared with this $x$=0.023 data in order to generate an estimate of the measurement's sensitivity. To give an initial sense of scale, the scattering volumes of the two samples were comparable and the $x$=0.023 sample's magnetic peak at (0.5, 0.5, 18) in Fig. S9 was collected at count times of 10 s/pt whereas the flat data for the $x$=0.05 sample in Fig. 4 (b) was collected at 270 s/pt. Using the normalized peak intensities and assuming the same theoretical spin structure for both $x$=0.023 and $x$=0.05, the upper bound for the AF ordered moment in the $x$=0.05 sample becomes $m_{AF} < 0.06\ \mu_B$. This number also accounts for the changes in the relative intensities of the weak (0.5, 0.5, odd) structural peaks induced via La-substitution (a factor of ~ 3.4 enhancement for $x$ = 0.05).

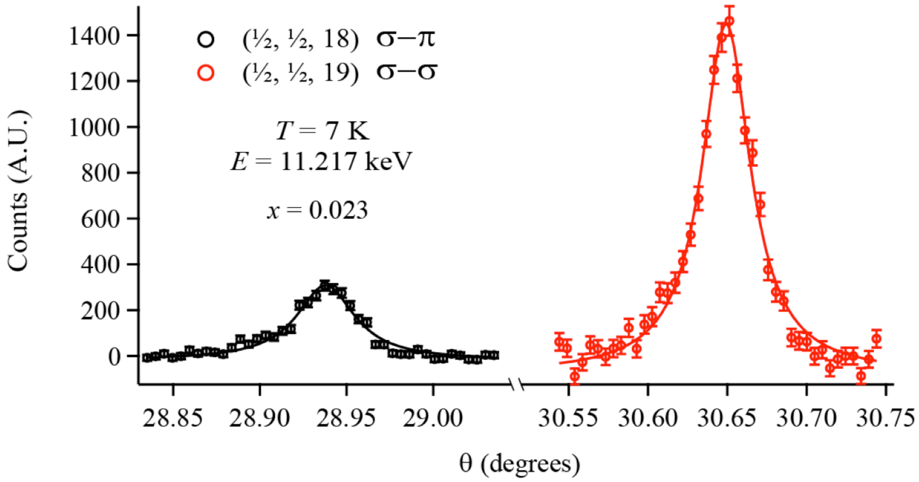


*Fig. S9: Theta-two theta scans of the (½, ½, 18) and (½, ½, 19) features in their respective scattering channels for a doped sample where both are present (x = 0.023). Solid lines depict Lorentzian fits of the peaks.*

**X. Magnetic Susceptibility of $Sr_3Ir_2O_7$**

To better illustrate the appearance of a Curie Weiss form of high temperature susceptibility in the La-doped $Sr_3Ir_2O_7$ samples, susceptibility data was collected for the undoped parent system in a Quantum Design Dynacool vibrating sample magnetometer under an applied field of $H$ = 2 T (Fig. S10). Above $T_N$ ~285 K, the high temperature response decreases linearly with a small slope with increasing temperature. This is consistent with results earlier reported by Nagai, *et al.* [27]. Attempts to fit this range of high temperature data to a form of Curie-Weiss behavior failed to converge.

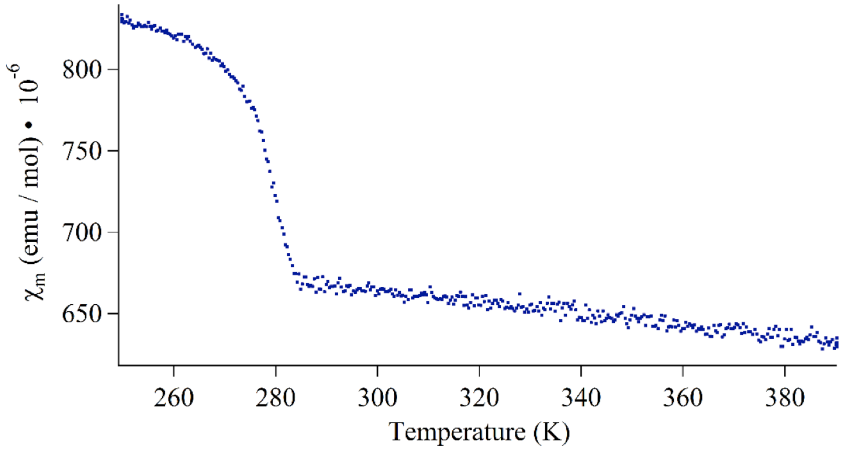


*Fig. S10: Magnetic molar susceptibility of $Sr_3Ir_2O_7$ showing a weak linear dependence above $T_N$. Data was collected while cooling under an applied H=2T.*

**References**

[21] M. Moretti Sala, V. Schnells, S. Boseggia, L. Simonelli, A. Al-Zein, J. G. Vale, L. Paolasini, E. C. Hunter, R. S. Perry, D. Prabhakaran, A. T. Boothroyd, M. Krisch, G. Monaco, H. M. Rønnow, D. F. McMorrow, and F. Mila. Phys. Rev. B 92, 024405 (2015).

[25] Tom Hogan, Z. Yamani, D. Walkup, Xiang Chen, Rebecca Dally, Thomas Z. Ward, John Hill, Z. Islam, Vidya Madhavan, and Stephen D. Wilson, Phys. Rev. Lett. 114, 257203 (2015).

[27] I. Nagai, Y. Yoshida, S. I. Ikeda, H. Matsuhata, H. Kito and M. Kosaka. J. Phys. Condens. Matter 19, 136214 (2007).
